# Supplementary material for: Diffusion in a $d$-dimensional rough potential
Source: arXiv:2508.04674 ancillary file (2026-06-17)
Supplement: Supplementary file 1 [file supplementals.pdf]

# 1 Supplementary Material

## 1.1 MFPT integrals

From

$$\mathbb{E}[T] = \int_0^\infty (1 - F(t)) dt \quad (1)$$

we can write

$$\mathbb{E}[T] = \int_0^\infty \left[ \frac{1}{\sqrt{4\pi\beta^2\sigma^2}} \int_0^\infty \frac{1}{\lambda} \exp\left(-\frac{(\ln \lambda + \beta\mu)^2}{4\beta^2\sigma^2} - \lambda t\right) d\lambda \right]^n dt \quad (2)$$

Let  $u = \ln \lambda$  in the inner integral:

$$\mathbb{E}[T] = \int_0^\infty \left[ \frac{1}{\sqrt{4\pi\beta^2\sigma^2}} \int_{-\infty}^\infty \exp(-\exp(u)t) \exp\left(-\frac{(u + \beta\mu)^2}{4\beta^2\sigma^2}\right) du \right]^n dt \quad (3)$$

Note the presence of the standard normal pdf  $f$ :

$$f(u \mid -\beta\mu, 2\beta^2\sigma^2) = \frac{1}{\sqrt{4\pi\beta^2\sigma^2}} \exp\left(-\frac{(u + \beta\mu)^2}{4\beta^2\sigma^2}\right) \quad (4)$$

Therefore:

$$\mathbb{E}[T] = \int_0^\infty \left[ \int_{-\infty}^\infty \exp(-\exp(u)t) f(u \mid -\beta\mu, 2\beta^2\sigma^2) du \right]^n dt \quad (5)$$

We can then evaluate the ratio  $\phi = \mathbb{E}[T] / \lim_{\beta^2\sigma^2 \rightarrow 0} \mathbb{E}[T]$ :

$$\begin{aligned} \phi &= \frac{\mathbb{E}[T]}{\lim_{\sigma^2 \rightarrow 0} \mathbb{E}[T]} = \frac{\int_0^\infty \left[ \int_{-\infty}^\infty \exp(-\exp(u)t) f(u \mid -\beta\mu, 2\beta^2\sigma^2) du \right]^n dt}{\int_0^\infty \left[ \int_{-\infty}^\infty \exp(-\exp(u)t) \lim_{\beta^2\sigma^2 \rightarrow 0} f(u \mid -\beta\mu, 2\beta^2\sigma^2) du \right]^n dt} \\ &= \frac{\int_0^\infty \left[ \int_{-\infty}^\infty \exp(-\exp(u)t) f(u \mid -\beta\mu, 2\beta^2\sigma^2) du \right]^n dt}{\int_0^\infty \left[ \int_{-\infty}^\infty \exp(-\exp(u)t) \delta(u + \beta\mu) du \right]^n dt} \\ &= \frac{\int_0^\infty \left[ \int_{-\infty}^\infty \exp(-\exp(u)t) f(u \mid -\beta\mu, 2\beta^2\sigma^2) du \right]^n dt}{\int_0^\infty \exp(-n \exp(-\beta\mu)t) dt} \\ &= n \exp(-\beta\mu) \int_0^\infty \left[ \int_{-\infty}^\infty \exp(-\exp(u)t) f(u \mid -\beta\mu, 2\beta^2\sigma^2) du \right]^n dt \end{aligned} \quad (6)$$

where we use the Gaussian definition of the Dirac-delta function, i.e.  $f(x \mid 0, \sigma^2) \rightarrow \delta(x)$  as  $\sigma^2 \rightarrow 0$ . Then, let  $v = u + \beta\mu$ :

$$\begin{aligned}
\phi &= n \exp(-\beta\mu) \int_0^\infty \left[ \int_{-\infty}^\infty \exp(-\exp(v - \beta\mu)t) f(v \mid 0, 2\beta^2\sigma^2) \, dv \right]^n \, dt \\
&= n \exp(-\beta\mu) \int_0^\infty \left[ \int_{-\infty}^\infty \exp(-\exp(v) \exp(-\beta\mu)t) f(v \mid 0, 2\beta^2\sigma^2) \, dv \right]^n \, dt
\end{aligned} \tag{7}$$

and the additional substitution  $\tau = \exp(-\beta\mu) t$ :

$$\phi = n \int_0^\infty \left[ \int_{-\infty}^\infty \exp(-\exp(v)\tau) f(v \mid 0, 2\beta^2\sigma^2) \, dv \right]^n \, d\tau \tag{8}$$

matching the expression in the main text, where  $f(v) = f(v \mid 0, 2\beta^2\sigma^2)$  for brevity.
